# Supplementary material for: Muon capture in nuclei: an ab initio approach based on quantum Monte Carlo methods
Source: arXiv:1903.08078 source file (2019-03-19)
Supplement: Supplementary file 1 [file supplemental.pdf]

# Muon capture in nuclei: an *ab initio* approach based on quantum Monte Carlo methods
# Supplemental Material

A. Lovato[a,b], N. Rocco[b,c], and R. Schiavilla[d,e]
[a] *INFN-TIFPA Trento Institute of Fundamental Physics and Applications, 38123 Trento, Italy*
[b] *Physics Division, Argonne National Laboratory, Argonne, IL 60439, USA*
[c] *Theoretical Physics Department, Fermi National Accelerator Laboratory, Batavia, IL 60510, USA*
[d] *Department of Physics, Old Dominion University, Norfolk, VA 23529, USA*
[e] *Theory Center, Jefferson Lab, Newport News, VA 23606, USA*
(Dated: March 8, 2019)

In this supplemental note we provide a more detailed account of the maximum-entropy techniques we utilize to obtain the response functions $R_{\alpha\beta}(q,\overline{\omega})$ from their imaginary-time counterparts $E_{\alpha\beta}(q,\tau)$. For notational simplicity, we drop below the subscripts $\alpha\beta$ and only keep the explicit dependence on $\overline{\omega}$ (or $\tau$).

According to Bayesian principles, the "most probable" response function is the one that maximizes $\Pr[R|E]$, the conditional probability of $R(\overline{\omega})$ given $E(\tau)$. Bayes theorem states that $\Pr[R|E] \propto \Pr[E|R] \times \Pr[R]$, where $\Pr[E|R] \propto \exp(-\chi^2/2)$ is the likelihood function and $\Pr[R]$ is the prior probability. Attempting an inversion of the Laplace transform by merely minimizing the $\chi^2$, and hence assuming that that $\Pr[R]$ is either unimportant or unknown, leads to unphysical oscillations of the reconstructed response function. Within the maximum entropy method, the response function, being positive definite and integrable, is interpreted as a probability distribution. As such, it maximizes the the entropy $S$ and a natural choice for the prior is $\Pr[R] \propto \exp(S)$.

The practical implementation of the scheme above proceeds as follows. We compute by GFMC methods a set of $N_E = 1280$ Euclidean response functions (a set for each value of the momentum transfer). A single Euclidean response function is obtained by averaging the independent unconstrained imaginary-time propagation of 2000 initial configurations. Hence, a total of 2,560,000 configurations are used (for each value of $q$), which allows us to control the Monte Carlo statistical error up to relatively large imaginary time. We employ a uniform grid in $\tau$ up to $\tau^{\max} = 0.1$ MeV$^{-1}$ with a spacing $\Delta\tau = 0.0005$ MeV$^{-1}$ (so $N_\tau = 200$ grid points $\tau_i$ between 0 and $\tau^{\max}$). The average Euclidean response function and covariance matrix are estimated as

$$\overline{E}_i = \frac{1}{N_E}\sum_{n=1}^{N_E} E_i^{(n)} \ , \tag{1}$$

$$C_{ij} = \frac{1}{N_E(N_E-1)}\sum_{n=1}^{N_E}\Big[\overline{E}_i - E_i^{(n)}\Big]\Big[\overline{E}_j - E_j^{(n)}\Big] \ . \tag{2}$$

where $E_i^{(n)} = E^{(n)}(\tau_i)$ is the Euclidean response function corresponding to the $n^{\rm th}$ GFMC propagation.

After discretizing the energy transfer variable $\overline{\omega}$ on $N_\omega$ evenly spaced points (spacing $\Delta\overline{\omega}$), the Laplace transform reported in Eq. (11) of the main article is expressed as

$$E_i = \sum_{j=1}^{N_\omega} K_{ij} R_j \ , \tag{3}$$

where $E_i = E(\tau_i)$, $R_j = R(\overline{\omega}_j)$, and $K_{ij} = \Delta\overline{\omega}\ \exp(-\overline{\omega}_j\tau_i)$ is the discretized Laplace kernel.

There is a high degree of correlation between subsequent time steps, since the imaginary-time evolution from one step to the next involves small changes in the space and spin-isospin amplitudes. As a consequence, the covariance matrix is non-diagonal, and the $\chi^2$ is given by

$$\chi^2 = \sum_{i,j=1}^{N_\tau}\left(\overline{E}_i - E_i\right)\left(C^{-1}\right)_{ij}\left(\overline{E}_j - E_j\right) \ . \tag{4}$$

Following Ref. [1], we diagonalize the covariance matrix so that $(\mathbf{U}^{-1}\mathbf{C}\mathbf{U})_{ij} = \delta_{ij}\,{\sigma'_i}^2$, and define the rotated kernel and data as, respectively, $\mathbf{K}' = \mathbf{U}^{-1}\,\mathbf{K}$ and $\overline{\mathbf{E}}' = \mathbf{U}^{-1}\,\overline{\mathbf{E}}$. In terms of these, the likelihood then reads

$$\chi^2 = \frac{1}{N_\tau}\sum_{i=1}^{N_\tau}\frac{(\sum_j K'_{ij}R_j - \overline{E}'_i)^2}{{\sigma'_i}^2} \ . \tag{5}$$

We also define the entropy of the distribution $R$ as

$$S = \sum_{i=1}^{N_\omega}\big[R_i - M_i - R_i\ln(R_i/M_i)\big]\Delta\overline{\omega} \ , \tag{6}$$

with $M_i = M(\overline{\omega}_i)$ being the *default model*. Note that the above expression is valid even when $R(\overline{\omega})$ and $M(\overline{\omega})$ have different normalizations.

In the context of maximum entropy techniques, the key step in the "inversion" of the Laplace transform is the minimization of $\alpha S - \chi^2/2$. To this end, we utilize the so-called "Brian algorithm" [2], a detailed discussion of which can also be found in the supplemental material of Ref. [3]. There, two non-informative default models for the prior

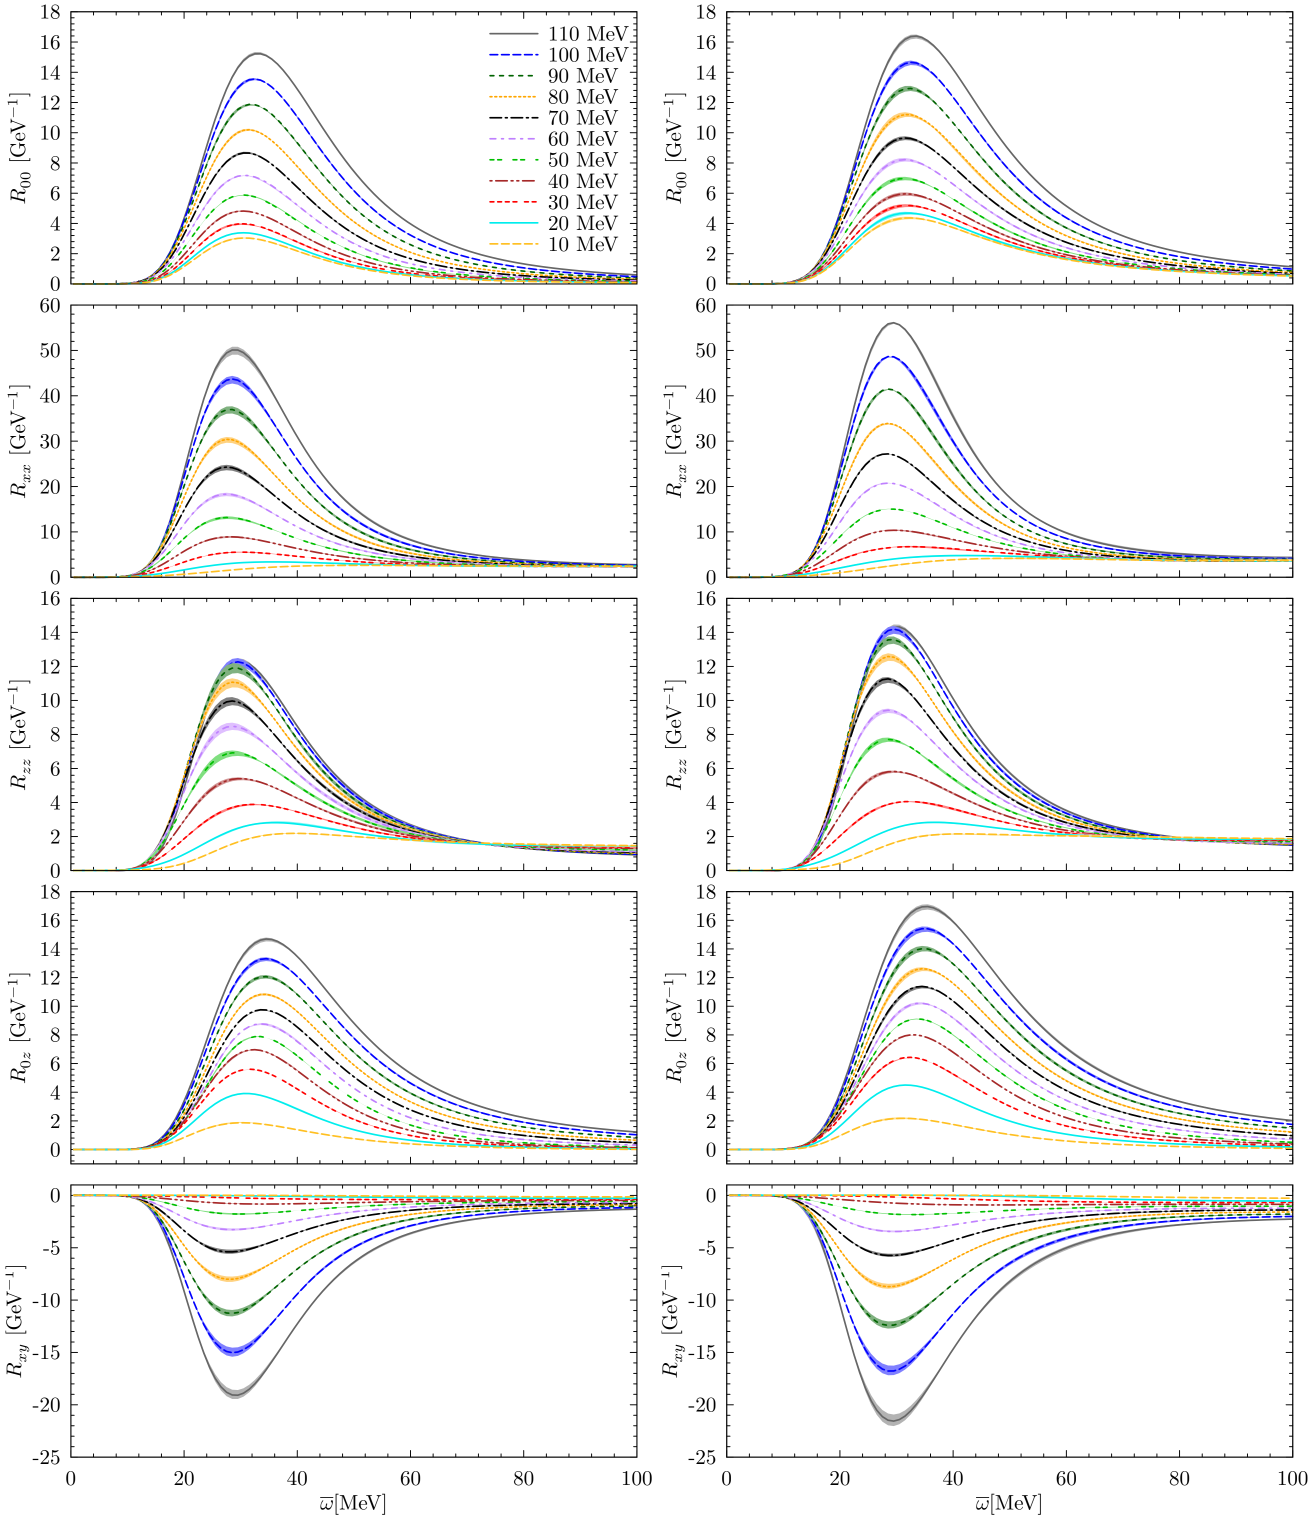


FIG. 1. Charged-current response functions of $^4$He at momentum transfers in the range $q = (10–110)$ MeV. The results obtained including one-body only and both one- and two-body terms in the weak current are displayed on the left (right) panels.

were considered: (i) a flat one $M_F(\overline{\omega}) \propto \theta(\overline{\omega}_M - \overline{\omega})$, where $\theta(\overline{\omega})$ is the step function and $\overline{\omega}_M = 2$ GeV, and (ii) a simple Gaussian $M_G(\overline{\omega}) \propto \exp(-\overline{\omega}^2/\sigma^2)$ with $\sigma$ as specified below.

The *historic* maximum entropy prescription was adopted in Ref. [3]. It consists in determining, for the parameter $\alpha$, the value $\alpha_{\rm h}$ in correspondence to which the minimum of $\alpha\, S - \chi^2/2$ occurs for $\chi^2 = 1$. The error bands shown in Ref. [3] reflected the change in the response functions associated with the two choices above of the prior. In a subsequent paper [4], a more refined strategy was devised to estimate the theoretical uncertainty in the electromagnetic response functions of $^{12}$C. Because of the substantial computational cost involved in evaluating the large number of response functions we utilize to map out the rate dependence on $E_\nu$, this latter procedure was deemed to be impractical here. Thus, in order to estimate this uncertainty, we simply compute the response functions corresponding to $\alpha = 2\,\alpha_{\rm h}$ and $\alpha = \alpha_{\rm h}/2$. We follow this procedure for both the flat and Gaussian prior; in the latter case, we take $\sigma = m_\mu \approx 105$ MeV.

In Fig. 1 we show the charged-current response functions of $^4$He for momentum transfer ranging from $q = 10$ MeV to $q = 110$ MeV. All response functions, but $R_{xy}$, turn out to be positive definite. Since the maximum entropy algorithm is only applicable to positive definite responses, we first flip the sign of $E_{xy}(\tau)$, then perform the inversion, and finally flip back the sign of the resulting $R_{xy}(\overline{\omega})$. The situation is slightly more complicated when only the axial contribution to the current operator is retained, since in that case $R_{0z}$ changes sign. We deal with this difficulty by adding to the original Euclidean response the Laplace transform of the positive definite distribution $\widetilde{R}_{0z}(\overline{\omega}) = c\,\theta(\overline{\omega} - \overline{\omega}_{\rm th})\,\theta(\overline{\omega}_M - \overline{\omega})$, where $\omega_{\rm th} \approx 19.8$ MeV is the breakup threshold of $^4$He into $^3$H$+n$. The constant $c$ is chosen so as to make the sum $R_{0z}(\overline{\omega}) + \widetilde{R}_{0z}(\overline{\omega})$ positive over the whole $\overline{\omega}$ domain. Once the inversion is performed, $\widetilde{R}_{0z}(\overline{\omega})$ is subtracted out. We explicitly verified that this procedure is stable against small variations in $c$.

When performing the inversion, no information on the location of the threshold is imposed, and the response functions are different from zero for $\overline{\omega} < \overline{\omega}_{\rm th}$. To remedy this shortcoming, one could evolve to much larger imaginary time, possibly up to $\tau^{\rm max} = 0.2$ MeV$^{-1}$. However, in order to reduce the statistical fluctuations associated with the fermion-sign problem, this would require increasing the already large set of configurations employed in the propagation, making the calculation considerably more computationally intensive than is already. On the other hand, we find that the total capture rate is rather insensitive to the choice of $\tau^{\rm max}$. Including one- and two-body terms in the weak current, we obtain $\Gamma = (303 \pm 21, 303 \pm 10, 306 \pm 9)$ s$^{-1}$ for $\tau^{\rm max} = (0.05, 0.08, 0.1)$ MeV$^{-1}$. Moreover, the integrated strength beyond the physical threshold varies as $(57 \pm 8, 42 \pm 3, 40 \pm 3)$ s$^{-1}$ as $\tau^{\rm max}$ is increased over the same range.

Finally, we note that the monotonic behavior exhibited by the responses as function of the momentum transfer simplifies the interpolation needed to compute the differential capture rate displayed in Fig. 1 of the main article.


[1] M. Jarrell and J. E. Gubernatis, Phys. Rept. **269**, 133 (1996).

[2] R. K. Bryan, European Biophysics Journal **18**, 165 (1990).

[3] A. Lovato, S. Gandolfi, J. Carlson, S. C. Pieper, and R. Schiavilla, Phys. Rev. **C91**, 062501 (2015), arXiv:1501.01981 [nucl-th].

[4] A. Lovato, S. Gandolfi, J. Carlson, S. C. Pieper, and R. Schiavilla, Phys. Rev. Lett. **117**, 082501 (2016), arXiv:1605.00248 [nucl-th].
